# Supplementary material for: Robust Perception-Based Navigation using PAC-NMPC with a Learned Value Function
Source: arXiv:2309.13171 source file (2025-06-10)
Supplement: Supplementary file 1 [file appendix.tex]

\section{Appendix}

\subsection{Modified PAC Bound}

In this paper, we used a modified PAC bound for the expected cost. Note that in Figure \ref{fig:pacbounds}, the expected cost is quite large. This is because the robot is often very far from the goal region and the learned value function itself can be very large. This is a problem for the PAC bound because its divergence term scales quadratically with the maximum sampled trajectory cost:
\begin{align}
  \mathcal{J}^+_\alpha(\vectg{\nu})\! &= \! \widehat{\mathcal J}_\alpha(\vectg{\nu}) + \alpha d(\vectg{\nu}) + \Phi_{\alpha}(\delta) \\
  d(\bnu)\! &= \! \frac{1}{2L}\sum_{i=0}^{L-1}b_i^2e^{D_2\left(p(\cdot | \bnu)||(p(\cdot | \bnu_i)\right)} \\
  0 &\leq J(\bX_{ij}) \leq b_i \; \forall j = 0, ..., M \label{eq:divergence_metric}
\end{align}
As a result, as the sampled costs get larger, the divergence term, $d(\bnu)$, scales much more quickly than the robust estimate, $\widehat{\mathcal J}_\alpha(\vectg{\nu})$, which results in very poor bounds. Here, we present a proof for an improved PAC bound.
\\
\begin{proof}
	\begin{align}
	\intertext{The PAC Bound guarantee from PAC-NMPC is:}           
	   \mathbb{P}&\left(\mathcal{J}(\bnu) \leq \mathcal{J}^+_\alpha(\bnu)\right) \geq 1 - \delta \label{eq:proof1}\\
  	\intertext{$\mathcal{J}(\bnu)$ is the expected cost}           
            \mathcal{J}(\bnu) &= \mathbb{E}_{\bX, \bU \sim p(\cdot, \cdot|\bnu)}\left[J(\bX)\right] \label{eq:proof2}\\
	\intertext{The PAC bound,  $\mathcal{J}^+_\alpha(\bnu)$, depends on costs of sampled trajectories, $J(\bX_{ij})_{\;\forall\:i,j}$. For clarity, I write that out explicitly}      
 		\mathcal{J}^+_\alpha(\bnu) &= \mathcal{J}^+_\alpha(\bnu,J(\bX_{ij})_{\;\forall\:i,j}) \label{eq:proof3}\\
        \intertext{Rewrite PAC Bound guarantee, eq. \ref{eq:proof1}, more explicitly given eq. \ref{eq:proof2} and eq. \ref{eq:proof3}}
		\mathbb{P}&\Biggl(\mathbb{E}_{\bX, \bU \sim p(\cdot, \cdot|\bnu)}\bigg[J(\bX)\bigg] \nonumber \\
            &\leq \mathcal{J}^+_\alpha(\bnu,J(\bX_{ij})_{\;\forall\:i,j})\Biggr) \geq 1 - \delta \\
        \intertext{If we normalize the costs of sampled trajectories with positive constant $w$, then optimize a bound using the normalized costs, we get the following bound:}
		\mathbb{P}&\Biggl(\mathbb{E}_{\bX, \bU \sim p(\cdot, \cdot|\bnu)}\bigg[\frac{1}{w}J(\bX)\bigg] \nonumber \\
            &\leq \mathcal{J}^+_\alpha(\bnu,\frac{1}{w}J(\bX_{ij})_{\;\forall\:i,j})\Biggr) \geq 1 - \delta \\
        \intertext{Multiply through by the normalization constant:}
		\mathbb{P}&\Biggl(w\mathbb{E}_{\bX, \bU \sim p(\cdot, \cdot|\bnu)}\bigg[\frac{1}{w}J(\bX)\bigg] \nonumber \\
            &\leq w\mathcal{J}^+_\alpha(\bnu,\frac{1}{w}J(\bX_{ij})_{\;\forall\:i,j})\Biggr) \geq 1 - \delta \\
        \intertext{Linearity of expectation: $\mathbb{E}[aX +b] = a\mathbb{E}[X] + b$}
		\mathbb{P}&\Biggl(\mathbb{E}_{\bX, \bU \sim p(\cdot, \cdot|\bnu)}\bigg[J(\bX)\bigg] \nonumber \\
            &\leq w\mathcal{J}^+_\alpha(\bnu,\frac{1}{w}J(\bX_{ij})_{\;\forall\:i,j})\Biggr) \geq 1 - \delta \\
        \intertext{Let $\mathcal{J}^+_{\alpha, w} = w\mathcal{J}^+_\alpha(\bnu,\frac{1}{w}J(\bX_{ij})_{\;\forall\:i,j})$}
		\mathbb{P}&\left(\mathcal{J}(\bnu) \leq \mathcal{J}^+_{\alpha, w}(\bnu)\right) \geq 1 - \delta
	\end{align}
\end{proof}

By strategically selecting $w$, we can obtain an improved PAC bound. Thus, in this paper, we optimize
\begin{align}
    \bnu^* &= \argmin_{\bnu}\min_{\alpha>0} (\mathcal{J}^+_{\alpha, w} + \gamma \mathcal{C}^+_\alpha(\bnu)) \\
    w &= \frac{1}{LM}\sum^{L-1}_{i=0}\sum^{M}_{j=0}J(\bX_{ij})
\end{align}

\textcolor{red}{What's the best way to include this in the paper?}

\subsection{Additional things to investigate}

\textcolor{red}{If we have time \& budget, here are additional things that we can investigate}
\begin{itemize}
    \item Compare against a global planner method (e.g. RRTx)
    \item Compare against a learned waypoint method
    \item Test out varying finite horizon lengths.
    \item Update the learned value function online
    \item Demonstrate robustness to model mismatch
\end{itemize}
